# Supplementary material for: Exact Combinatorial Optimization with Temporo-Attentional Graph Neural Networks
Source: arXiv:2311.13843 source file (2023-11-23)
Supplement: Supplementary file 1 [file 10_supplementary.tex]

{\huge Supplementary Materials\\}

Here we provide details on how to create benchmarks in this paper. We also reveal training and evaluation procedure that we have adopted in our paper. 
% \footnote{\yong{Code is included in the supplementary materials package.}}  
\footnote{\yong{Code is available at:\\ \url{https://drive.google.com/drive/folders/1yrA4DETuBZH-RLntgNPLgHI7iVy_fIFe?usp=sharing}
}}

\section{More Details on the Datasets}
As stated in the paper we evaluate our results on 6 different benchmarks, the MILP instances of which span a fair spectrum of difficulty amongst the available MILP benchmarks. 
\begin{itemize}
    \item{Benchmark 1, Set Covering (SC):} with 1000 variables generated based on the work of Balas and Ho \cite{balas1980set}. Following \cite{gasse2019exact} we train on easy MILP samples with only 500 constraints, and evaluate the trained model on the MILP instances with 500 (Easy), 1000 (Medium), and 1500 (Hard) constraints.
    % \vspace{-4pt}
    \item{Benchmark 2, Combinatorial Auctions (CA):} Similar to \cite{gasse2019exact} we train on instances with 100 variables (items) vs 500 constraints (bids), and evaluate the trained model on three sets of Easy, Medium and Hard problems representing item-bid pairs of (100, 500), (200, 1000), and (300, 1500) respectively. This dataset is generated according to \cite{leyton2000towards}.
    % \vspace{-4pt}
    \item{Benchmark 3, Capacitated Facility Locations (CFL):} generated using the method in \cite{cornuejols1991comparison} with 100 variables (facilities). The Easy, Medium, and Hard problems each have 100, 200 and 400 constraints (customers), respectively. As a routine procedure, we train on easy samples and evaluate on the three mentioned MILP instance categories regarding their level of difficulty.
    % \vspace{-4pt}
    \item{Benchmark 4,  Maximum Independent Set (MIS):} generated according to \cite{bergman2016decision}. It is consist of maximum independent set instances on Erd\"os-R\'{e}nyi random graphs \cite{gasse2019exact}, with affinity set to 4. Similar to the previous benchmarks we train on Easy samples with 500 nodes and evaluate on instances with 500 (Easy), 1000 (Medium) and 1500 (Hard) nodes.
    % \vspace{-4pt}
    \item{Benchmark 5, work load appointments (Load balancing (LB)):} This dataset represents data associated to allocating workloads (data streams/computational assignments) to the minimum number of workers (\eg servers/GPU clusters) possible. This dataset contains 9900 train, 100 validation, and 100 test MILP instances \cite{ml4co_gasse}. 
    % \vspace{-4pt}
    \item{Benchmark 6, Maritime Inventory Routing (MIR):} The MILP instances associated to this dataset are created according to publicly released information on global bulk shipping \cite{papageorgiou2014mirplib}. This benchmark contains 98 train, 20 validation and 20 test MILP instances. 
    % \vspace{-4pt}
\end{itemize}

\section{Training}
We train our neural brancher on the samples generated by recording $L$ consecutive episodes of a MILP branching decision process. In particular for each MILP instance we choose the native full strong branching (FSB) of SCIP as our expert agent. The features associated to each node and edge at each branching state are extracted by the environment and represented by a bipartite graph. Each bipartite graph encodes information about the current node's LP relaxation, dual and primal bounds, previous decision on the fractional variables  etc. On the other hand, the FSB expert, based on such environmental information selects an action $\tilde{a}_t$ from an action set $\mathcal{A}_t\subset\{1,\ldots,p\}$, where $p$ is the number of variables that must satisfy the integrality constraint. The action will be the variable index on which the FSB expert branches. We record the groups of $L$ consecutive branching episodes for each MILP instance, which contain the bipartite graph $(\mathcal{G},\bfC_t,\bfV_t,\bfE_t)$ along with the FSB expert action for each episode. At the training time a cross entropy loss minimizes the distribution distance between the model predictions and these actions as the ground truth labels. 

We train our policy with an Adam \cite{kingma2014adam} optimizer with $lr=.001$ and the PyTorch's native \texttt{ReduceLROnPlateau} scheduler with patience of 10 epochs and reduction rate of .2, that reduces the learning rate if the model has stopped improving. We train for 50 epochs and validate on the validation set. We use PreNorm layers as described in \cite{gasse2019exact} to normalize the input graph features.

\begin{figure*}[htb!]
\centering
   \includegraphics[width=.9\linewidth]{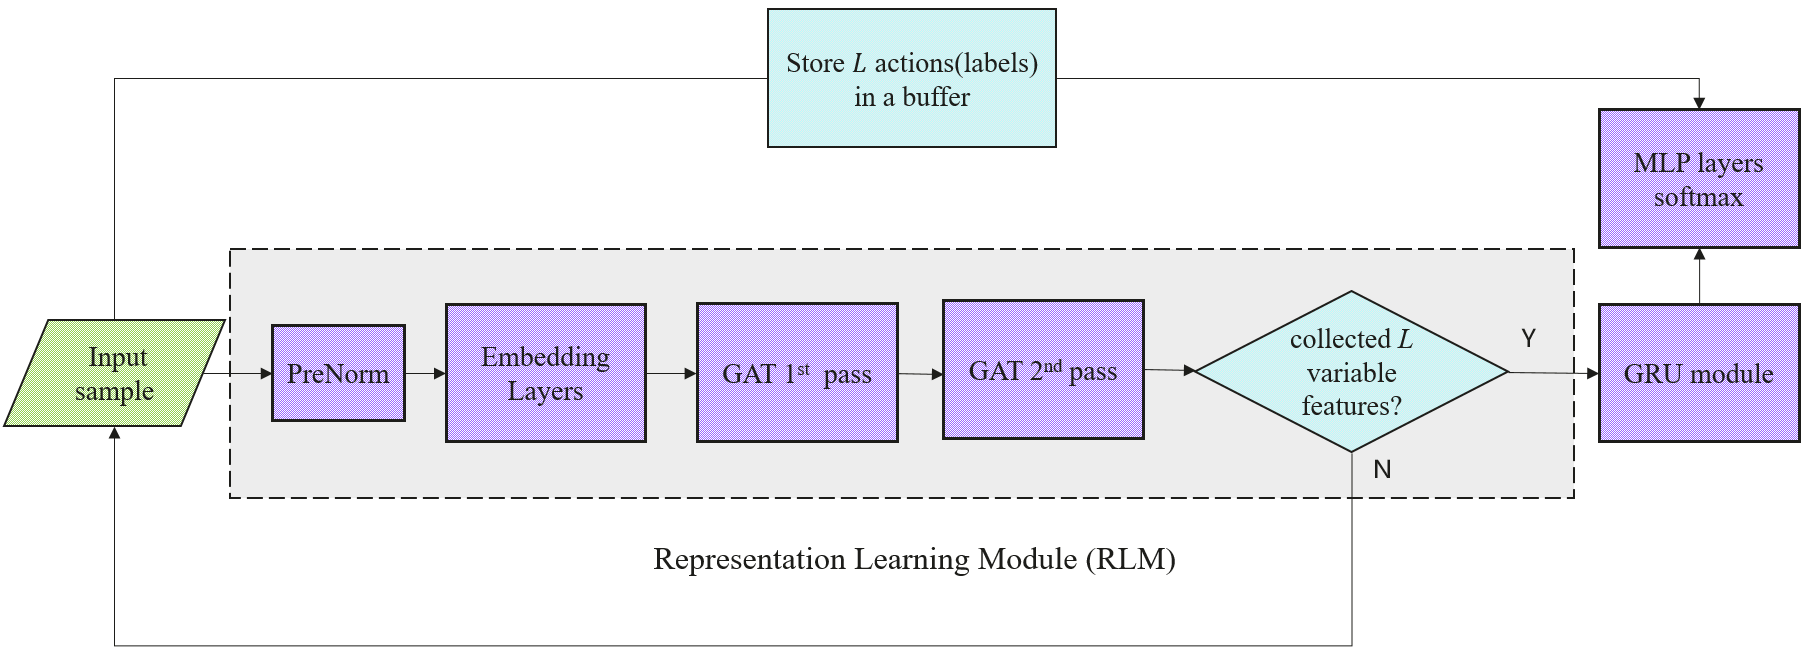}
\caption{Training Scheme for our proposed Temporo-Attentional mechanism. Bipartite representations of $L$ consecutive states associated to successive branching episodes of a MILP instance are fed to the training module. The associated FSB expert actions are used as ground truth labels.}
\label{fig:training_scheme}
\end{figure*}

The Representation Learning Module (RLM) in Figure \ref{fig:training_scheme}, functions like a Siamese network \cite{chicco2021siamese} with $L$ bipartite graphs as input. The graphs are fed to the RLM in a batch of $L$ samples. The RLM eventually reproduces a representation vector $\bfv_{i,t}~\forall (i,t):1\leq i\leq n, t -L + 1\leq t$. The $L$ successive representation vectors associated to each variable node are then fed into the GRU and then an MLP layer with a softmax head for branching predictions.
Figure \ref{fig:system_module} describes the training scenario using the Siamese network concept. The models connected with dashed lines share weights.

\begin{figure*}[htb]
\centering
   \includegraphics[width=.6\linewidth]{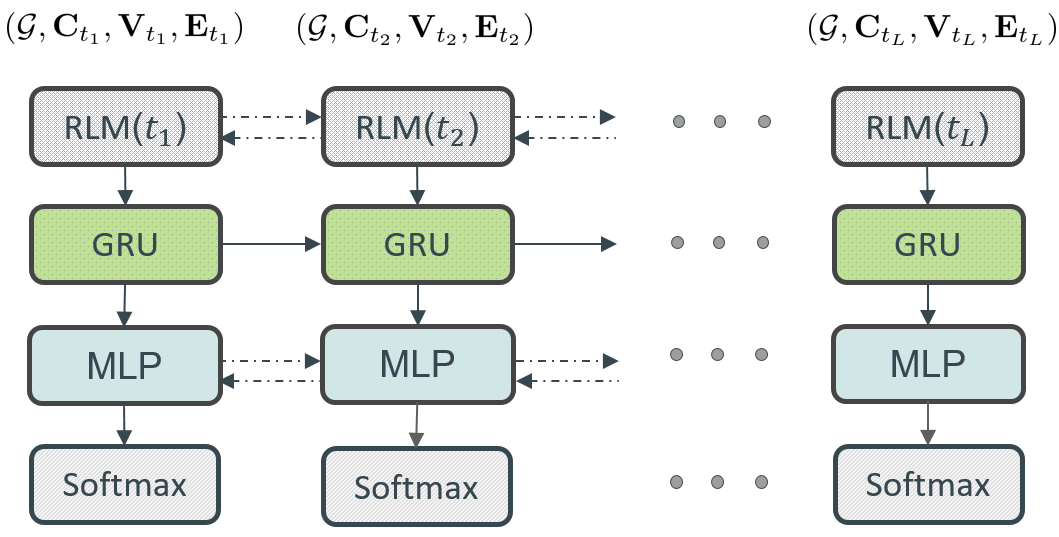}
\caption{Siamese presentation of our proposed training scheme. The RLM is the two pass attentional message passing module. The RLM and MLP layers for all the $L$ consecutive samples share common weights.}
\label{fig:system_module}
\end{figure*}

\section{Inference}
At the inference time, initially our method needs $L-1$ bipartite graph representations from the environment to start predicting the $L^{\rm th}$ branching action from the action set provided by the solver environment. Therefore, in the first $L-1$ episodes the branching process associated to each MILP instance, we utilize one of the internal branching rules as our branching agent. Once the first $L-1$ episodes are solved, our proposed TGAT policy acts as the agent in the remaining episodes of the branching Markov process. In our experiments we get SCIP's internal pseudo-cost brancher (PB) to help solving the first $L-1$ MILP nodes associated to each MILP instance. Figure \ref{fig:inference_schematic}, references to our proposed inference hybrid technique for solving MILP instances.

\begin{figure*}[htb!]
\centering
   \includegraphics[width=.9\linewidth]{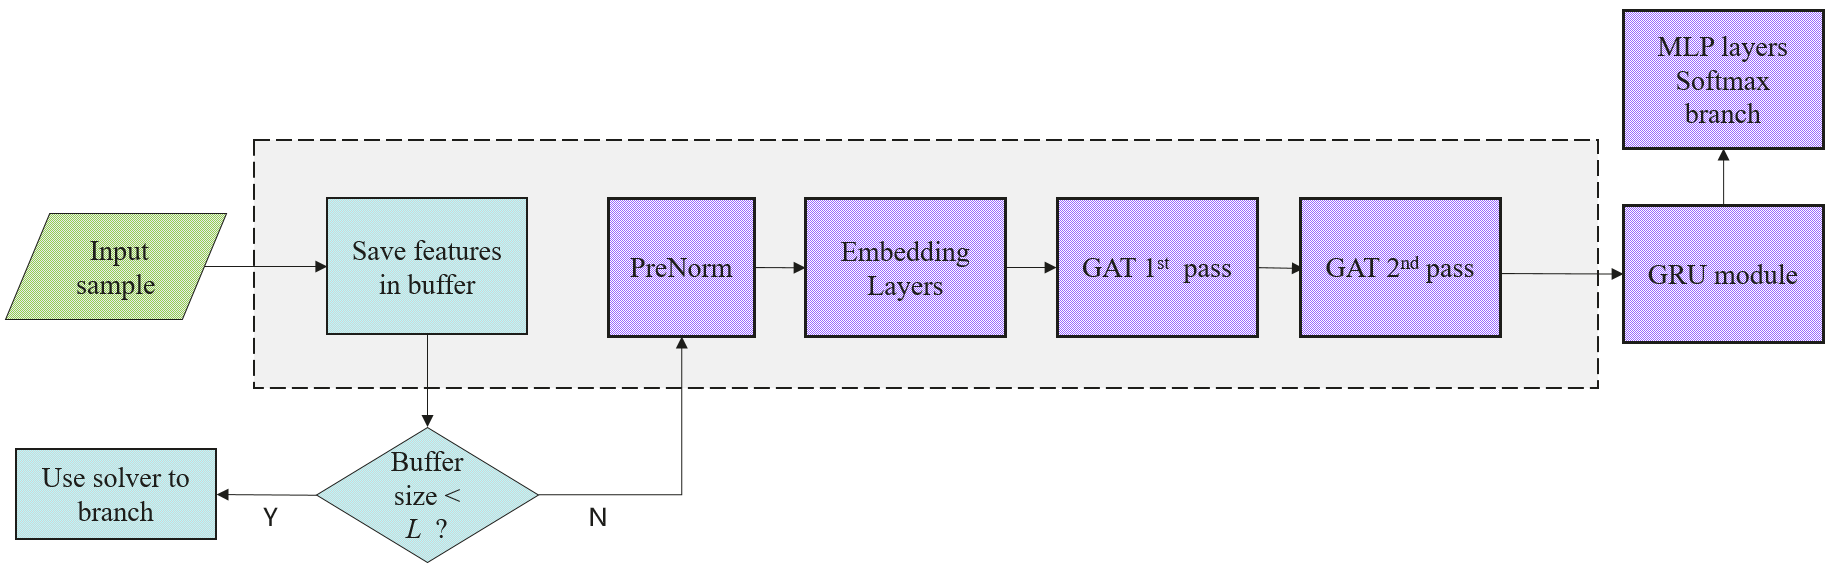}
\caption{Inference flow in our proposed TGAT scheme.}
\label{fig:inference_schematic}
\end{figure*}

\section{Ablation Studies}
\subsection{GRU Sequence Length $L$}

% \begin{wrapfigure}{r}{0.4\textwidth}
\begin{figure}[htb!]
\centering
   \includegraphics[width=.6\linewidth]{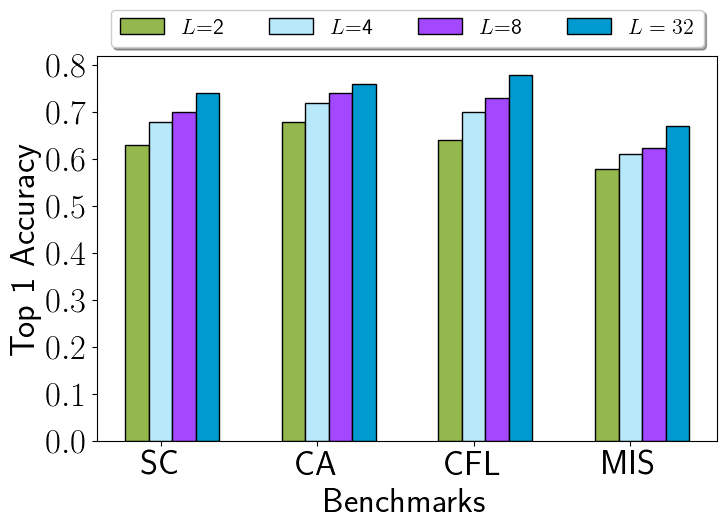}
\caption{Effect of increasing the sequence length $L$ in the validation set top-1 accuracy across 4 benchmarks. As $L$ increases our policy performs better in imitating the FSB expert brancher.}
\label{fig:ablation_L}
% \end{wrapfigure}
\end{figure}

In this section we study the effect of increasing the sequence length $L$ in our policy performance for the Set Covering (SC), Combinatorial Auctions (CA), Capacitated Facility Locations (CFL) and Maximum Independent Set (MIS) benchmarks. Figure \ref{fig:ablation_L}, shows the top-1 validation accuracy of our propose TGAT method with respect to the sequence length $L$. It can be deduced from this figure that the length $L$ and the top-1 accuracy are directly proportional, which in turn means, the branching quality of our trained model increases as more historical samples are considered. 

Additionally Table \ref{tab:reward_ablation_L}, shows the dual-integral reward associated to policies trained on each benchmark with different sequence length $L$. As it can be seen there is no canonical rule applicable to the inference branching performance across our benchmarks. The reason is that although increasing the sequence length $L$ helps the model to do a more accurate branching job at each node, it adds to the model complexity at the same time. The number of parameters associated to the GRU structure in our model is directly dependent to the sequence length; therefore, the inference time for the policies with longer sequence lengths will increase. 

\begingroup
\setlength{\tabcolsep}{1.5pt} % Default value: 6pt
 % Default value: 1
\begin{table*}[htb!]
\centering
\scriptsize
{
    \caption{Ablation on the sequence length $L$ in terms of Dual Integral Reward for time-limit of 3600s and $H=2$, where larger reward is better. The optimal length for each benchmark is different due to the complexity of its underlying MILP instances.}
    \centering
    \begin{tabular}{c}
         \Xhline{2\arrayrulewidth}
        \begin{tabular}{l|cccccc}
            \multirow{2}{*}{\backslashbox{Benchmark}{Method}} & GCNN & GAT & TGAT & TGAT & TGAT & TGAT\\
            & & & ($L=2)$ & ($L=4)$ & ($L=8)$ & ($L=32)$ \\
            % GCNN&GAT&TGAT($L=2)$&TGAT($L=4)$&TGAT($L=8)$&TGAT($L=32)$\\    
             \Xhline{1\arrayrulewidth}
             Set Covering&  1,048,019 &  1,085,403 & 1,090,105 & 1,092,453 & 1,086,920 & 1,083,255\\
             Combinatorial Auctions&   -53,470,516 & -53,232,134 & -53,358,279& -53,458,279& -53,468,603 & -53,582,421\\
             Cap. Facility Locations & 76,457,625 & 76,497,211  & 76,568,953 &  76,521,205 & 76,456,925 &76,317,495\\
             Max. Independent Set&  -1,640,797 & -1,635,131 & -1,632,623&  -1,628,261&  -1,640,668& -1,642,428\\
                          \Xhline{1\arrayrulewidth}
        \end{tabular}
    \end{tabular}
    \label{tab:reward_ablation_L}
}
\end{table*}
\endgroup

\begingroup
\setlength{\tabcolsep}{3pt} % Default value: 6pt
 % Default value: 1
\begin{table*}[htb!]
\centering
\scriptsize
{
    \caption{Ablation on the number of attention heads $H$ when the sequence length $L=2$ and solving time-limit is set to 3200 seconds.}
        % \vspace{.2cm}
    \vspace{0pt}
    \centering
    \begin{tabular}{c}
         \Xhline{2\arrayrulewidth}
        \begin{tabular}{l|cccc}
            % \backslashbox{Benchmark}{Parameters}& GCNN&TGAT($H=1)$&TGAT($H=2)$&TGAT($H=3)$\\

            \multirow{2}{*}{\backslashbox{Benchmark}{Method}} & GCNN & TGAT & TGAT & TGAT \\
            & & ($H=1)$ & ($H=2)$ & ($H=3)$ \\

             \Xhline{1\arrayrulewidth}
            Set Covering& 1,048,019  & 1,086,668  & 1,090,105 & 1,090,685\\
            Combinatorial Auctions&-53,470,516 &-53,359,124 &-53,358,279&-53,471,532\\
            Capacitated Facility Locations&76,457,625 & 76,478,321 &76,568,953 & 76,497,211\\
            Maximum Independent Set& -1,640,797  &-1,639,912  &-1,632,623 &-1,638,214\\
              \Xhline{1\arrayrulewidth}
        \end{tabular}
    \end{tabular}
    \label{tab:reward_ablation_H}
}
\end{table*}
\endgroup

\begingroup
\setlength{\tabcolsep}{3pt} % Default value: 6pt
 % Default value: 1
\begin{table*}[htb!]
\centering
\scriptsize
{
    \caption{Ablation on the embedding size $d$ for the first 4 benchmarks in terms of the dual integral reward with solving time-limit of 3600s and $H=2$ and $L=2$.}
    \centering
    \begin{tabular}{c}
         \Xhline{2\arrayrulewidth}
        \begin{tabular}{l|cccc}
            % \backslashbox{Benchmark}{Parameters}& GCNN($d=64$)&GCNN($d=32$)&TGAT($d=64)$&TGAT($d=32)$\\    
            \multirow{2}{*}{\backslashbox{Benchmark}{Method}} & GCNN & GCNN & TGAT & TGAT\\
            & ($d=64)$ & ($d=32)$ & ($d=64)$ & ($d=32)$ \\
             \Xhline{1\arrayrulewidth}
            Set Covering& 1,048,019  & 1,049,121 & 1,880,123  & 1,090,105 \\
            Combinatorial Auctions&-53,470,516 &-53,471,216&-53,401,281  &-53,358,279\\
            Capacitated Facility Locations&76,457,625 &76,456,132   & 76,493,531&76,568,953\\
            Maximum Independent Set& -1,640,797  &-1,641,321&-1,633,425  &-1,632,623 \\
              \Xhline{1\arrayrulewidth}
        \end{tabular}
    \end{tabular}
    \label{tab:ablation_emb}
}
\end{table*}
\endgroup

Since our metric looks at the branching quality in terms of decreasing the dual gap, as well as the rate at which the branchings are performed (fast policies); increasing the sequence length might hurt the performance. Therefore, in this situation we should look for a trade-off point  between higher branching accuracy and faster policy.
\subsection{GAT Number of Attention Heads $H$}
In this sub-section we study the effect of number of attention heads on the performance of our policy. 

% \begin{wrapfigure}{r}{0.4\textwidth}
\begin{figure}[htb!]
\centering
   \includegraphics[width=.6\linewidth]{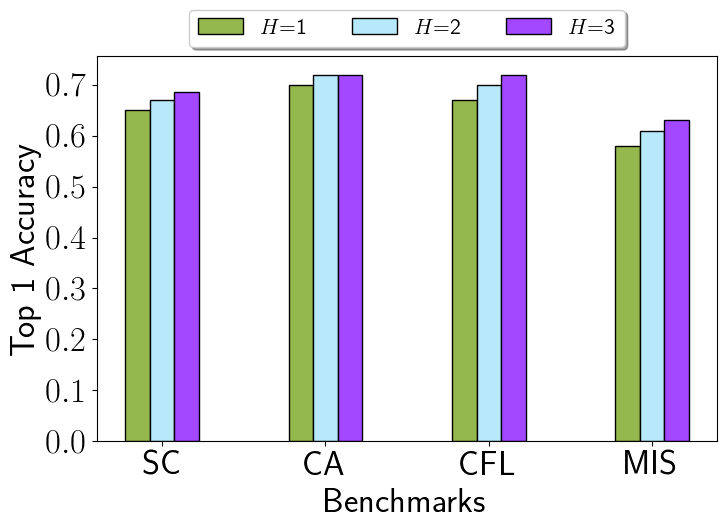}
\caption{Effect of increasing the number of attention heads $H$, in the validation set top-1 accuracy across 4 benchmarks. As $H$ increases our policy performs better in imitating the FSB expert brancher.}
\label{fig:ablation_H}
% \end{wrapfigure}
\end{figure}

As Figure \ref{fig:ablation_H} shows the validation accuracy increases if the number of attention heads is increased as a result of increasing the capacity of the model. However, increasing the capacity may increase the risk of overfitting in rather easy datasets like combinatorial auctions. Therefore, increasing the number of attention heads may not always be beneficial. 
Table \ref{tab:reward_ablation_H} also shows the dual integral reward associated to the ablation study on $H$ when the sequence length $L$ is fixed and set to $2$ for a solving time-limit of 3600 seconds. As this table suggests, increasing the number of attention heads depending to the benchmark may or may not increase the branching performance. For larger MILP instances like those of set covering benchmark, increasing the number of attention heads helps; however, for smaller MILP instances like combinatorial auctions increasing $H$ may not benefit the reward much or even hurt the performance. Therefore, the number of attention heads should be tuned as a hyper-parameter depending to the underlying benchmark.

\subsection{Embedding Size}
Embedding size, also like the sequence length $L$ or the number of attention heads $H$, plays an important role in the model capacity. As Table \ref{tab:ablation_emb} shows, in general, we have achieved a better performance when using $d=32$ as opposed to $d=64$ when attention mechanism is enabled; however, for the GCNN baseline decreasing the embedding size to 32 may hurt the performance in some cases. Generally speaking, the model capacity should be enough to capture the solver behaviour. If the embedding size is too high then the model overfits and at the same time at the inference the model latency hurts the performance. If the model is too small it underfits in the training time and although the inference latency is decreased, the dual integral reward may get hurt due to smaller gap leaps per solving an LP node. 

\begingroup
\setlength{\tabcolsep}{8pt} % Default value: 6pt
 % Default value: 1
\begin{table*}[htb!]
\centering
\scriptsize
{
    \caption{Ablation on different parameters of the attention module in terms of the dual integral reward with solving time-limit of 3600s and $H=2$ and $L=4$.}
    % \vspace{.2cm}
    % \vspace{-8pt}
    \centering
    \begin{tabular}{c}
         \Xhline{2\arrayrulewidth}
        \begin{tabular}{ccccc}
             Share Weight &Dropout & Self Loop& Concat& Reward\\    
             \Xhline{1\arrayrulewidth}
             \xmark& \xmark&\cmark&\xmark&112,934,222 \\
             \cmark& \xmark&\cmark&\xmark&110,234,421 \\
             \xmark& \cmark&\cmark&\xmark&112,843,135 \\
             \xmark& \xmark&\cmark&\cmark&111,124,729 \\
             \xmark& \xmark&\xmark&\xmark&109,436,527 \\
              
              \Xhline{1\arrayrulewidth}
        \end{tabular}
    \end{tabular}
    \label{tab:ablation_attn_diff}
}
\end{table*}
\endgroup

% \begingroup
% \setlength{\tabcolsep}{2pt} % Default value: 6pt
% \renewcommand{\arraystretch}{1} % Default value: 1
% \begin{table*}[htb!]
% \centering
% \scriptsize
% {
%     \caption{Average dual integral reward plus standard deviation percentage across 5 experiment runs with different seeds. We use the $(d,H,L)$ notation presented in the paper for the TGAT structure for each benchmark.}
%         % \vspace{.2cm}
%     % \vspace{-8pt}
%     \centering
%     \begin{tabular}{c}
%          \Xhline{2\arrayrulewidth}
%         \begin{tabular}{l|cccccc}
%             TGAT&SC(32,2,4)&CA(32,2,2) &CFL(32,2,2)&MIS(32,2,4) &LB(32,3,4)&MIR(32,2,4)\\    
%              \Xhline{1\arrayrulewidth}
%              Reward & $1,092,453 \pm .65\%$ & $-53,358,279\pm .00\%$  & $76,568,953\pm .32\%$ & $-1,628,261\pm .14\%$ & $2,529,981\pm .53\%$ & $112,934,222\pm 1.2\%$ \\
%         \end{tabular}
%     \end{tabular}
%     \label{tab:ablation_seed}
% }
% \end{table*}
% \endgroup

\begingroup
\setlength{\tabcolsep}{2pt} % Default value: 6pt
 % Default value: 1
\begin{table*}[htb!]
\centering
\scriptsize
{
    \caption{Average dual integral reward plus standard deviation percentage across 5 experiment runs with different seeds. We use the $(d,H,L)$ notation presented in the paper for the TGAT structure for each benchmark.}
        % \vspace{.2cm}
    % \vspace{-8pt}
    \centering
    \begin{tabular}{c}
         \Xhline{2\arrayrulewidth}
        \begin{tabular}{l|c}
            TGAT & Reward \\
            \Xhline{1\arrayrulewidth}
            SC(32,2,4) & $1,092,453 \pm .65\%$ \\
            CA(32,2,2) & $-53,358,279\pm .00\%$ \\
            CFL(32,2,2) & $76,568,953\pm .32\%$ \\
            MIS(32,2,4) & $-1,628,261\pm .14\%$ \\
            LB(32,3,4) & $2,529,981\pm .53\%$ \\
            MIR(32,2,4) & $112,934,222\pm 1.2\%$\\    
        \end{tabular}
    \end{tabular}
    \label{tab:ablation_seed}
}
\end{table*}
\endgroup

\subsection{Other Parameters of Attention}
In this section we ablate on different other parameters of the attention module when $H=2$ and $L=2$ for the maritime inventory routing dataset. These parameters include
\begin{itemize}
    \item Sharing weights: In this case the model weights $\Theta^{(h)}$ and $\Psi^{(h)}$ for variables, constraints, and edge features, in (1) to (4) share same parameters across different attention heads.
    \item Dropout: If set to \texttt{True} then $\alpha$ and $\beta$ in (2) and (4) will be subjected to a dropout layer with probability $p$ and become: $\alpha^{h} = \textrm{Dropout}(\alpha^{(h)},p)$, and $\beta^{h} = \textrm{Dropout}(\beta^{(h)},p).$ We use $p=.2$ in this study.
    \item Self loops: If set to \texttt{False} then the self loops in (1) and (3) will be removed. Particularly in this case $\alpha_{ii}^{(h)} = \beta_{jj}^{(h)} = 0$.
    \item Concat: If set to $\texttt{True}$, then embeddings $\bfc_{i,t}$ and $\bfv_{i,t}$ in (1) and (3) will be concatenated instead of averaged. The associated model parameters dimensions will change accordingly. 
\end{itemize}
Table \ref{tab:ablation_attn_diff} shows different setups of such parameters. In general for maritime routing inventory dataset, sharing parameters cause the model to underfit; thereby, decreases the policy reward. In this case the reduction in the inference time cannot compensate the reduction in the model branching accuracy due to weight sharing. Dopout layers also do not provide any benefits. Concatentating the features from different attention heads in this experiment causes the model capacity to increase as a result of adding to the model parameters. This on one hand causes the model to overfit, and on the other hand adss to the model complexity and hence, increases the solving time. Finally, Removing the self loop also hurts the performance of the policy which suggests that self attention matters in MILPs.
\subsection{Effect of Different Seeds}
In this section we report the aggregated results of the dual integral reward for different benchmarks over 5 experiment runs for different randomizing seeds. Our SCIP environment as well as other optimization solver suites use a randomization parameter \emph{seed} specially at the beginning of each MILP episode to break the tie between some internal mechanisms used in the environment of such solvers \cite{gasse2019exact}.
We report the effect of such randomization in the dual integral reward in Table \ref{tab:ablation_seed}. Specifically we report $\mu\pm \sigma/\mu\times 100$ where $\mu$ is the mean dual integral reward and $\sigma$ is the standard deviation across different runs. We have seen the maximum deviation in the results for the maritime inventory routing dataset.

\section{Future Works}
A future research could be expanding our work to proposing a generic dataset independent model that can perform reasonably well across a fair number of benchmarks. To that end, utilizing unsupervised methods as well as techniques that are known to the domain adaptation society come in handy.
